# Supplementary material for: Evaluating and Improving the Coreference Capabilities of Machine Translation Models
Source: arXiv:2302.08464 source file (2023-02-16)
Supplement: Supplementary file 1 [file 04_models_exampels.tex]

\input{tables/lang_exampels}
In Table \ref{table:lang_exampels_app} we show translation examples in Spanish and French that demonstrate unique features in each language. Two such unique phenomena that affect our methodology are the pronoun drop in Spanish and the effect of possessive pronouns and French. In the examples, we show a translation of a WinoMT sentence from WinoMT where the pronoun is dropped. The second examples show a translation where the aligned pronoun is a possessive pronoun, which in French has the gender of the possessed noun and not the gender of the possessor. In both those cases, we can get a correct translation without information concerning the aligned pronoun gender. This is the reason we exclude those cases from our evaluation.

The first example in Table \ref{table:lang_exampels_app} shows a French translation where the aligned pronoun is a verb. These cases show how our methodology can correctly identify translations where the aligned pronoun belongs to other parts of speech. This ability is a clear advantage over the previous method that either looks for an exact match with a known target pronoun or either really on a set of predefined translation alternatives, as Both methods can easily miss such cases. We note that this effect occurs in a wide range of languages and even more so in partial pro-drop languages.

\begin{table*}[ht]
% \begin{tabular}{lll}
\centering
\resizebox{1\textwidth}{!}{
\begin{tabular}{p{7cm}p{7.5cm}p{0.5cm}}
\toprule
Source & {[}Target lang.{]} Predicted translation &  \\
  \midrule
\parbox{7cm}{Bob would rather fill his emergency fund using his \textcolor{orange}{mobile} instead of the \textcolor{orange}{bank} because \textcolor{orange}{it} was closed.} &
  \parbox{7.5cm}{{[}FR.{]} Bob préférerait remplir son fonds d'urgence en utilisant son \textcolor{blue}{mobile} au lieu de la \textcolor{red}{banque} parce \textcolor{blue}{qu'il} était fermé.} &
  % \parbox{5cm}{ In the baseline translation to French the pronoun have different gender than the coreferring entity} \\
    \textbf{\textcolor{red}{\xmark}} \\
  \midrule
\parbox{7cm}{Bob would rather fill his emergency fund using his \textcolor{orange}{mobile} instead of the <ENT1> \textcolor{orange}{bank} </ENT1> because <ENT1> \textcolor{orange}{it} </ENT1> was closed.} &
  \parbox{7.5cm}{{[}FR.{]} Bob préférerait remplir son fonds d'urgence en utilisant son \textcolor{blue}{téléphone} portable au lieu de la \textcolor{red}{banque} parce \textcolor{red}{qu'elle} était fermée.} &
  % \parbox{5cm}{ Our model translation to French have the same gender to the pronoun and the coreferring entity} \\
    \textbf{\textcolor{greenrgb}{\cmark}} \\
  % \bottomrule

  \midrule
  \parbox{7cm}{The headphones blocked the \textcolor{orange}{noise} but not the \textcolor{orange}{vibration}, as \textcolor{orange}{it} was relatively strong.}
  &
  \parbox{7.5cm}{{{[}RU.{]} \foreignlanguage{russian}{Наушники блокировали \textcolor{blue}{шум}, но не \textcolor{red}{вибрацию}, поскольку \textcolor{blue}{он} был относительно сильным.}}} &
  \textbf{\textcolor{red}{\xmark}} \\
  \midrule
  \parbox{7cm}{The headphones blocked the \textcolor{orange}{noise} but not the <ENT1> \textcolor{orange}{vibration} </ENT1>, as <ENT1> \textcolor{orange}{it} </ENT1> was relatively strong.} &
  \parbox{7.5cm}{{{[}RU.{]} \foreignlanguage{russian}{Наушники блокировали \textcolor{blue}{шум}, но не \textcolor{red}{вибрацию}, так как \textcolor{red}{она} была относительно сильной.}}} &
  \textbf{\textcolor{greenrgb}{\cmark}} \\
  \bottomrule
\end{tabular}
}
\caption{Examples of sentences from our datasets and their translations. Those translation examples show a case where the baseline model fails to generate the correct translation, but our model succeeds. Words in blue,
red, and orange indicate male, female and neutral entities, respectively.}
\label{table:lang_improve_app}
\end{table*}

In Table \ref{table:lang_improve_app} we show other examples where our fine tuning approach improves the quality of the translation.
