# Supplementary material for: Evaluating and Improving the Coreference Capabilities of Machine Translation Models
Source: arXiv:2302.08464 source file (2023-02-16)
Supplement: Supplementary file 3 [file 02_bleu_results.tex]

% Please add the following required packages to your document preamble:
% \usepackage[table,xcdraw]{xcolor}
% If you use beamer only pass "xcolor=table" option, i.e. \documentclass[xcolor=table]{beamer}
\begin{table}[h!]
\centering
\resizebox{\columnwidth}{!}{
\begin{tabular}{lrrrrrr}
\toprule
%  &
%   \multicolumn{1}{c}{German} &
%   \multicolumn{1}{c}{Spanish} &
%   \multicolumn{1}{l}{French} &
%   \multicolumn{1}{l}{Russian} &
%   \multicolumn{1}{c}{Hebrew} &
%   \multicolumn{1}{c}{Arabic} \\
&
  \multicolumn{1}{c}{de} &
  \multicolumn{1}{c}{es} &
  \multicolumn{1}{l}{fr} &
  \multicolumn{1}{l}{ru} &
  \multicolumn{1}{c}{he} &
  \multicolumn{1}{c}{ar} \\
\midrule
Opus-MT        & 32.6 & 29.0 & 34.2 & 26.8 & 40.0 & 21.2 \\
% random\_text\_g & 32.656 & 28.5723 & 34.1957 & 26.435  & 35.78 & 24.69 \\
gender data  & 32.6 & 28.6 & 34.2 & 26.2 & 36.0 & 23.2 \\
$+$coref markers        & 32.4 & 28.6   & 34.1 & 26.2 & 35.9 & 23.0 \\
\bottomrule
\end{tabular}}
\caption{BLEU results of our fine tuning approaches on OPUS test data.}
\label{table:bleu}
\end{table}

Table \ref{table:bleu} show BLEU (sacrebleu \citep{post-2018-call}\footnote{\url{https://github.com/mjpost/sacrebleu}}) results for our approaches. We calculated those results on the Opus test data of each language. We can notice that in most languages the models have only a minor change in BLEU results after fine tuning. An exception for that is Hebrew and Arabic that few points increase or decrease in their results. The reason for that can be the existence of only one test dataset for those languages in Opus test data.
