# Supplementary material for: Evaluating and Improving the Coreference Capabilities of Machine Translation Models
Source: arXiv:2302.08464 source file (2023-02-16)
Supplement: Supplementary file 4 [file 03_bug_results.tex]

% Please add the following required packages to your document preamble:
% \usepackage[table,xcdraw]{xcolor}
% If you use beamer only pass "xcolor=table" option, i.e. \documentclass[xcolor=table]{beamer}
\begin{table*}[tb!]
\centering
\begin{tabular}{lrrrrrr}
\toprule
%  &
%   \multicolumn{1}{c}{German} &
%   \multicolumn{1}{c}{Spanish} &
%   \multicolumn{1}{l}{French} &
%   \multicolumn{1}{l}{Russian} &
%   \multicolumn{1}{c}{Hebrew} &
%   \multicolumn{1}{c}{Arabic} \\
 &
  \multicolumn{1}{c}{en$\rightarrow$de} &
  \multicolumn{1}{c}{en$\rightarrow$es} &
  \multicolumn{1}{l}{en$\rightarrow$fr} &
  \multicolumn{1}{l}{en$\rightarrow$ru} &
  \multicolumn{1}{c}{en$\rightarrow$he} &
  \multicolumn{1}{c}{en$\rightarrow$ar} \\
\midrule
mBART50         & 74.6 & 69.4 & 76.0 & 69.1 & 80.2 & 83.0 \\
M2M\_418M       & 81.3 & 84.9 & 86.0 & \textbf{71.6} & 83.6 & 85.1 \\
M2M\_1.2B       & \textbf{83.5} & 85.1 & \textbf{90.3} & 70.4 & \textbf{89.6} & \textbf{93.4} \\
Google          & 56.0 & 84.4 & 89.2 & 71.0 & 85.2 & 91.9 \\
Microsoft       & 77.2 & \textbf{86.7} & 86.0 & 67.2 & 84.0 & 89.8 \\
Opus-MT         & 79.8 & 85.1 & 86.2 & 67.3 & 88.8 & 88.0 \\

% mBART50   & \textbf{77.7} & \textbf{75.2} & \textbf{73.3} & 57.7 & \textbf{69.3} & \textbf{69.5} \\
% M2M\_418M & 69.7 & 55.1 & 65.4 & 54.7 & 56.5 & 64.3 \\
% M2M\_1.2B & 69.9 & 59.4 & 65.5 & 57.9 & 60.1 & 69.2 \\
% Google         & 79.9 & 73.4 & 70.2 & \textbf{60.0}   & 66.6 & 64.2 \\
% Microsoft      & 78.0   & 66.5 & 69.3 & 57.3 & 63.9 & 60.7 \\
% Opus-MT       & 68.2 & 56.0   & 63.2 & 49.8 & 59.0   & 59.8 \\
% random data    & 68.2 & 59.2 & 66   & 65.4 & 67.8 & 64.5 \\
% coref data     & 75.1 & 60.6 & 68.3 & 61.6 & 68.1 & 66.2 \\
% +signal       & 78.5 & 60.1 & 68.6 & 58.4 & 69   & 60.9 \\
% +gold         & 79.3 & 60   & 69.1 & 60.9 & 68.5 & 62.7 \\
\bottomrule
\end{tabular}
\caption{Target-side consistency results of commercial and open-source MT on BUG when translating into different languages. These numbers are an upper bound for the source-side coreference accuracy.}
%\gabis{consider merging with Table~\ref{table:gmf_cons_winox}}}
\label{table:gmf_cons_BUG}
\end{table*}

% % Please add the following required packages to your document preamble:
% % \usepackage[table,xcdraw]{xcolor}
% % If you use beamer only pass "xcolor=table" option, i.e. \documentclass[xcolor=table]{beamer}
% \begin{table}[]
% \begin{tabular}{lrrrrrr}
%  &
%   \multicolumn{1}{c}{de} &
%   \multicolumn{1}{c}{es} &
%   \multicolumn{1}{c}{fr} &
%   \multicolumn{1}{c}{ru} &
%   \multicolumn{1}{c}{he} &
%   \multicolumn{1}{c}{ar} \\
%  &
%   \multicolumn{1}{l}{\cellcolor[HTML]{FFFFFF}} &
%   \multicolumn{1}{l}{\cellcolor[HTML]{FFFFFF}} &
%   \multicolumn{1}{l}{\cellcolor[HTML]{FFFFFF}} &
%   \multicolumn{1}{l}{\cellcolor[HTML]{FFFFFF}} &
%   \multicolumn{1}{l}{\cellcolor[HTML]{FFFFFF}} &
%   \multicolumn{1}{l}{\cellcolor[HTML]{FFFFFF}} \\
% mBART50         & 74.6 & 69.4 & 76   & 69.1 & 80.2 & 83   \\
% M2M100\_\_418M  & 81.3 & 84.9 & 86   & 71.6 & 83.6 & 85.1 \\
% M2M100\_1.2B    & 83.5 & 85.1 & 90.3 & 70.4 & 89.6 & 93.4 \\
% Google          & 56   & 84.4 & 89.2 & 71   & 85.2 & 91.9 \\
% Microsoft       & 77.2 & 86.7 & 86   & 67.2 & 84   & 89.8 \\
% EasyNMT         & 79.8 & 85.1 & 86.2 & 67.3 & 88.8 & 88   \\
% random\_data    & 81.8 & 88.1 & 86.8 & 69.2 & 89.3 & 90.5 \\
% gender data     & 84.1 & 87.4 & 88.7 & 69.9 & 90.2 & 91.3 \\
% "+coref signal  & 84.2 & 87.4 & 88.8 & 70.1 & 89.8 & 91.8 \\
% "+gender signal & 82.2 & 0    & 86.5 & 66.6 & 0    & 0   
% \end{tabular}
% \end{table}
\input{tables/BUG/09_ours_cons}

%Table \ref{table:gmf_cons_BUG} present BUG consistency results of our baselines. The consistency results of BUG tend to be higher than results on Wino-X and WinoMT. A possible explanation can be the difference in the data characteristics. While every sentence in Wino-X and WinoMT is designed to have a distracting entity that the model can treat as the coreferring entity to the pronoun,  BUG sentences are naturalistic and usually don't have other entities that can confuse the model. This can allow MT model to benefit from one-to-one translation and achieve high consistency without solving the coreference. 

Table \ref{table:gmf_cons_BUG} present BUG consistency results of our baselines. The consistency results of BUG tend to be higher than results on Wino-X and WinoMT. A possible explanation can be that in BUG, an MT model can benefit from one-to-one translation and achieve high consistency without solving the coreference as the additional entities in each sentences are less distracting to the model than in the syntactic Wino-X and WinoMT.

%An interesting consequence of that explanation can be the effect on models performances. 
Nevertheless, BUG can be difficult to coreference resolvers as it contains long naturalistic sentences that may effect their performances. 

Table \ref{table:ours_cons_BUG} present the consistency results of our fine tuning approach on BUG. Our implicit data augmentation fine tuning on Gender data shows some improvement to the consistency results, and the explicit fine tuning with coreference markers shows additional moderate improvements.
