# Supplementary material for: Evaluating and Improving the Coreference Capabilities of Machine Translation Models
Source: arXiv:2302.08464 source file (2023-02-16)
Supplement: Supplementary file 11 [file 04_models_exampels.tex]

\input{tables/lang_exampels}
Table \ref{table:lang_exampels_app} shows translation examples from English to Spanish and French that demonstrate unique features in each language. The first example shows a French translation where the gender of the pronoun is reflected by the feminine inflection of the verb ``giflée''. This demonstrates how our methodology can successfully identify translations where the aligned pronoun belongs to other parts of speech than pronouns. We note that this effect occurs in a wide range of languages and even more so in partial pro-drop languages.

The second example shows a French translation that contains a possessive pronoun, which does not indicate the gender of the possessor. The last example shows a Spanish translation where the pronoun is omitted. In both last cases, we can get a correct translation without information concerning the aligned pronoun gender, we therefore exclude them from the evaluation.

\begin{table*}[ht]
% \begin{tabular}{lll}
\centering
\resizebox{1\textwidth}{!}{
\begin{tabular}{p{7cm}p{7.5cm}p{0.5cm}}
\toprule
Source & {[}Target lang.{]} Predicted translation &  \\
  \midrule
\parbox{7cm}{Bob would rather fill his emergency fund using his \textcolor{orange}{mobile} instead of the \textcolor{orange}{bank} because \textcolor{orange}{it} was closed.} &
  \parbox{7.5cm}{{[}FR.{]} Bob préférerait remplir son fonds d'urgence en utilisant son \textcolor{blue}{mobile} au lieu de la \textcolor{red}{banque} parce \textcolor{blue}{qu'il} était fermé.} &
  % \parbox{5cm}{ In the baseline translation to French the pronoun have different gender than the coreferring entity} \\
    \textbf{\textcolor{red}{\xmark}} \\
  \midrule
\parbox{7cm}{Bob would rather fill his emergency fund using his \textcolor{orange}{mobile} instead of the <ENT1> \textcolor{orange}{bank} </ENT1> because <ENT1> \textcolor{orange}{it} </ENT1> was closed.} &
  \parbox{7.5cm}{{[}FR.{]} Bob préférerait remplir son fonds d'urgence en utilisant son \textcolor{blue}{téléphone} portable au lieu de la \textcolor{red}{banque} parce \textcolor{red}{qu'elle} était fermée.} &
  % \parbox{5cm}{ Our model translation to French have the same gender to the pronoun and the coreferring entity} \\
    \textbf{\textcolor{greenrgb}{\cmark}} \\
  % \bottomrule

  \midrule
  \parbox{7cm}{The headphones blocked the \textcolor{orange}{noise} but not the \textcolor{orange}{vibration}, as \textcolor{orange}{it} was relatively strong.}
  &
  \parbox{7.5cm}{{{[}RU.{]} \foreignlanguage{russian}{Наушники блокировали \textcolor{blue}{шум}, но не \textcolor{red}{вибрацию}, поскольку \textcolor{blue}{он} был относительно сильным.}}} &
  \textbf{\textcolor{red}{\xmark}} \\
  \midrule
  \parbox{7cm}{The headphones blocked the \textcolor{orange}{noise} but not the <ENT1> \textcolor{orange}{vibration} </ENT1>, as <ENT1> \textcolor{orange}{it} </ENT1> was relatively strong.} &
  \parbox{7.5cm}{{{[}RU.{]} \foreignlanguage{russian}{Наушники блокировали \textcolor{blue}{шум}, но не \textcolor{red}{вибрацию}, так как \textcolor{red}{она} была относительно сильной.}}} &
  \textbf{\textcolor{greenrgb}{\cmark}} \\
  \bottomrule
\end{tabular}
}
\caption{Examples of sentences from our datasets and their translations. Those translation examples show a case where the baseline model fails to generate the correct translation, but our model succeeds. Words in blue,
red, and orange indicate male, female and neutral entities, respectively.}
\label{table:lang_improve_app}
\end{table*}

In Table \ref{table:lang_improve_app} we show other examples where our fine tuning approach improves the quality of the translation.
