# Supplementary material for: Evaluating and Improving the Coreference Capabilities of Machine Translation Models
Source: arXiv:2302.08464 source file (2023-02-16)
Supplement: Supplementary file 13 [file 06_data_sizes.tex]

% \input{tables/data/val}
% \input{tables/data/train}

% Table \ref{table:data_val} shows the number of instances in each evaluation dataset. Table \ref{table:data_train} shows the the size of Coref and Gender data for all six target languages.
